# Supplementary material for: Ditto in the House: Building Articulation Models of Indoor Scenes through Interactive Perception
Source: arXiv:2302.01295 source file (2023-02-02)
Supplement: Supplementary file 1 [file appendix.tex]

\section*{APPENDIX}

Appendixes should appear before the acknowledgment.

\section*{ACKNOWLEDGMENT}

The preferred spelling of the word ÒacknowledgmentÓ in America is without an ÒeÓ after the ÒgÓ. Avoid the stilted expression, ÒOne of us (R. B. G.) thanks . . .Ó  Instead, try ÒR. B. G. thanksÓ. Put sponsor acknowledgments in the unnumbered footnote on the first page.
